# Supplementary material for: Intelligent Software Tooling for Improving Software Development
Source: arXiv:2310.10921 source file (2023-10-17)
Supplement: Supplementary file 1 [file appendixA.tex]

\chapter{First Appendix with Awesome Data}
\label{appendixA}

%-----------------------------------
\section{Awesome Appendix Section}
\label{appendixA:sec1}
%-----------------------------------
